# Supplementary material for: Teaching VLMs to Localize Specific Objects from In-context Examples
Source: arXiv:2411.13317 source file (2025-03-12)
Supplement: Supplementary file 1 [file supp_data_mix.tex]

\begin{table*}[h]
    \centering
    
    \setlength{\tabcolsep}{6pt} % Adjust column spacing
    \begin{tabular}{l c c c c c}
        \toprule
        \textbf{Dataset} & \textbf{Shots} & \textbf{All Data} & \textbf{LASOT} & \textbf{GOT} & \textbf{TAO} \\
        \midrule
        PDM & 1 & \textbf{28.41} & 17.84 & 20.53 & 14.1 \\
         & 2 & \textbf{21.74} & 15.31 & 16.39 & 10.0 \\
                 \midrule

        PerSeg & 1 & \textbf{42.43} & 30.19 & 25.57 & 30.05 \\
        & 2 & \textbf{41.15} & 37.67 & 33.11 & 28.03 \\
        & 3 & \textbf{39.85} & 37.92 & 26.4 & 27.23 \\
        & 4 & 33.08 & \textbf{36.89} & 24.28 & 27.67 \\
                \midrule

        ICL-LASOT & 1 & \textbf{49.01} & 43.44 & 36.41 & 23.77 \\
         & 4 & 22.22 & \textbf{24.47} & 10.99 & 10.03 \\
         & 8 & 21.19 & \textbf{22.99} & 10.05 & 8.38 \\
                 % \midrule

        % ICL-LASOT fake & 1 & \textbf{44.04} & 41.37 & 27.05 & 16.95 \\
        %  & 4 & 20.65 & \textbf{21.19} & 8.85 & 8.77 \\
        %  & 8 & 16.39 & \textbf{21.3} & 9.34 & 8.1 \\
        \bottomrule
    \end{tabular}
    \caption{Ablation of data mixes}
    \label{tab:datamix_shots}
\end{table*}
