# Supplementary material for: Teaching VLMs to Localize Specific Objects from In-context Examples
Source: arXiv:2411.13317 source file (2025-03-12)
Supplement: Supplementary file 3 [file supp_llava_ov_train.tex]

\begin{table*}[t!]
    \centering
    
    \setlength{\tabcolsep}{10pt}
    \begin{tabular}{l c c c c}
        \toprule
        \textbf{Dataset} & \textbf{Shots} & \textbf{\llava OV} & \textbf{\llava OV trained} \\
        \midrule
        pdm & 1 & 1.27 & 0.43\\
        & 2 & 0.00 & 0.39\\
        \midrule
        perseg & 1 & 4.78 & 4.29\\
        & 2 & 0.00 & 2.99\\
        & 3 &  0.00 & 4.89 \\
        & 4 &  0.00 & 0.26\\
        \midrule
        LASOT & 1 & 1.10 &  1.86\\
        & 4 & 0.00 &  2.06\\
        & 8 & 0.00 & 0.46\\
        \bottomrule
    \end{tabular}
    \caption{Comparison of \% IoU LLaVa-OV with and without our training}
    \label{tab:miou_llava_ov_trained}
\end{table*}
