# Supplementary material for: Teaching VLMs to Localize Specific Objects from In-context Examples
Source: arXiv:2411.13317 source file (2025-03-12)
Supplement: Supplementary file 4 [file supp_prompt_big_models.tex]

\begin{table*}[t!]
    \centering
    
    \setlength{\tabcolsep}{6pt}
    \begin{tabular}{l c | c c c c | c c c c}
        \toprule
        & & \multicolumn{4}{c|}{\textbf{InternVL2-76B}} & \multicolumn{4}{c}{\textbf{Qwen2-VL-72B}} \\
        \textbf{Dataset} & \textbf{Shots} & \textbf{Prompt 0} & \textbf{Prompt 1} & \textbf{Prompt 2} & \textbf{Prompt 3} & \textbf{Prompt 0} & \textbf{Prompt 1} & \textbf{Prompt 2} & \textbf{Prompt 3} \\
        \midrule
        pdm & 1 & 23.28 & 27.48 & 31.26 & 29.11 & 33.65 & 16.88 & 19.96 & 21.23 \\
        pdm & 2 & 14.20 & 21.87 & 28.67 & 20.85 & 32.37 & 12.97 & 13.11 & 12.29 \\
        \midrule
        perseg & 1 & 34.51 & 49.01 & 50.01 & 46.06 & 0.81 & 41.88 & 44.75 & 34.91 \\
        perseg & 2 & 24.18 & 41.16 & 51.46 & 42.30 & 0.90 & 35.47 & 28.19 & 28.68 \\
        perseg & 3 & 44.94 & 43.22 & 49.37 & 50.03 & 0.29 & 49.51 & 43.43 & 45.50 \\
        perseg & 4 & 36.57 & 34.63 & 45.70 & 42.34 & 1.26 & 39.96 & 37.36 & 31.04 \\
        \midrule
        LASOT & 1 & 40.67 & 42.47 & 47.68 & 46.07 & 4.82 & 42.66 & 43.14 & 43.01 \\
        LASOT & 2 & 23.21 & 45.61 & 42.90 & 43.76 & 0.40 & 38.05 & 40.04 & 37.65 \\
        LASOT & 4 & 31.72 & 39.71 & 38.90 & 38.86 & 1.63 & 33.54 & 31.29 & 31.38 \\
        LASOT & 8 & 21.65 & 21.74 & 27.21 & 29.18 & 0.76 & 31.17 & 22.81 & 27.23 \\
        \midrule
        Avg.  &   & 29.49 & 36.69 & 41.32 & 38.86 & 7.69 & 34.21 & 32.41 & 31.29 \\
        \bottomrule        
    \end{tabular}
    \caption{Comparison of \% IoU for "big" models according to the instruction}
    \label{tab:big_models_prompt}
\end{table*}
