# Supplementary material for: Teaching VLMs to Localize Specific Objects from In-context Examples
Source: arXiv:2411.13317 source file (2025-03-12)
Supplement: Supplementary file 5 [file supp_seedbench_ablation.tex]

% \begin{table}[h!]
% \centering
% \begin{tabular}{|l|cccccccccc}
% \toprule
%  & Overall & Instance Attributes & Instance Identity & Instance Interaction & Instance Location & Instances Counting & Scene Understanding & Spatial Relation & Text Understanding & Visual Reasoning \\
% \midrule
% Baseline & 0.76 & 0.79 & 0.79 & 0.70 & 0.72 & 0.71 & 0.80 & 0.62 & 0.73 & 0.79 \\
% Ours (LORA FT)    & 0.75 & 0.78 & 0.78 & 0.70 & 0.70 & 0.70 & 0.80 & 0.58 & 0.71 & 0.79 \\
% Ours (Full FT)    0.002 & 0.000 & 0.000 & 0.000 & 0.000 & 0.012 & 0.000 & 0.000 & 0.000 & 0.000 \\
% \bottomrule
% \end{tabular}
% \caption{Qwen SeedBench-Image variants results}
% \label{table:seedbench_results}
% \end{table}

\begin{table*}[h!]
\centering

\setlength{\tabcolsep}{10pt}
\begin{tabular}{lccc}
\toprule
\textbf{Metric} & \textbf{Qwen2-VL 7B} & \textbf{Ours Real + Fake (LORA FT)} & \textbf{Ours Real + Fake (Full FT)} \\
\toprule
Overall & 76.41 & 75.41 & 00.21 \\
\midrule
Instance Attributes & 78.77 & 77.84 & 00.02 \\
Instance Identity & 79.46 & 78.37 & 00.00 \\
Instance Interaction & 70.10 & 70.10 & 00.00 \\
Instance Location & 72.09 & 69.73 & 00.00 \\
Instances Counting & 71.15 & 69.76 & 01.19 \\
Scene Understanding & 79.61 & 79.70 & 00.00 \\
Spatial Relation & 61.64 & 58.30 & 00.00 \\
Text Understanding & 72.62 & 71.43 & 00.00 \\
Visual Reasoning & 79.46 & 79.15 & 00.00 \\
\bottomrule
\end{tabular}
\caption{Qwen SeedBench-Image variants results}
\label{table:abl:seedbench_results}
\end{table*}
